# Supplementary material for: Chiral Bogoliubons in Nonlinear Bosonic Systems
Source: arXiv:1503.08824 source file (2015-03-30)
Supplement: Supplementary file 1 [file supp_mat.pdf]

# Supplemental Material for "Chiral Bogoliubons in Nonlinear Bosonic Systems"

Charles-Edouard Bardyn,[1] Torsten Karzig,[1] Gil Refael,[1] and Timothy C. H. Liew[2]

[1] *Institute for Quantum Information and Matter, Caltech, Pasadena, California 91125, USA*

[2] *Division of Physics and Applied Physics, Nanyang Technological University 637371, Singapore*

## TIGHT-BINDING MODEL FOR BOGOLIUBONS ON A KAGOME LATTICE

In this section, we construct and solve the tight-binding model presented in the main text, which provides a qualitative description of Bogoliubov excitations that "live" in a potential with minima forming a Kagome lattice and vortices/antivortices in the lattice plaquettes. In the tight-binding limit, we can model the Bogoliubov equation (3) of the main text with only three parameters: a diagonal on-site energy term $\Omega$ (obtained by solving for the eigenstates of $\omega_d(-i\nabla) - \omega_0 + 2\alpha|\psi_0(\mathbf{x})|^2 + V(\mathbf{x})$), a hopping term $t$ (determined by the interplay of the potential depth and the kinetic term), and an off-diagonal on-site term $ge^{i\phi(\mathbf{r})}$ which couples the components $u$ and $v$. The latter carries the phase of $\phi_0$. Assuming that the triangular unit cell (defined in Fig. 2b of the main text) contains an antivortex, we choose $\arg(\phi_0(A,B,C)) = (0, -2\pi/3, 2\pi/3)$ and therefore $\phi(A,B,C) = (0, 2\pi/3, -2\pi/3)$, with sites $A, B, C$ of the unit cell defined as in Fig. 2b of the main text.

With the above definitions, the tight-binding approximation of the Bogoliubov equation can be cast into a model of bosons $\hat{u}_i$ and $\hat{v}_i$ hopping on a Kagome lattice, as described by the non-unitary "Hamiltonian"

$$H_{TB} = \sum_i \left(\Omega \hat{u}_i^\dagger \hat{u}_i - \Omega \hat{v}_i^\dagger \hat{v}_i + g\mathrm{e}^{i\phi_i} \hat{u}_i^\dagger \hat{v}_i - g\mathrm{e}^{-i\phi_i} \hat{v}_i^\dagger \hat{u}_i\right) - t \sum_{\langle ij \rangle} \left(\hat{u}_j^\dagger \hat{u}_i - \hat{v}_j^\dagger \hat{v}_i\right). \tag{1}$$

As mentioned in the main text, the non-unitary form of the Bogoliubov equation (and $H_{TB}$) can lead to eigenvalues with an imaginary part which, if positive, correspond to unstable Bogoliubov excitations.

### Effective Haldane model

For weak coupling $g$, particle- and hole-like Bogoliubov excitations ($u$ and $v$) are described by an effective Haldane model on a Kagome lattice. Time-reversal symmetry breaking (via non-trivial hopping phases) is induced by virtual transitions between the components $u$ and $v$. In particular, in the limit $\Omega \gg t \gg g$, second-order perturbation theory in $g$ leads to the following correction for the hopping term in the sector $u$:

$$\sum_{\langle ij \rangle} \hat{u}_j^\dagger \left(g\mathrm{e}^{i\phi_j}\right) \frac{1}{2\Omega} (t) \frac{1}{2\Omega} \left(-g\mathrm{e}^{-i\phi_i}\right) \hat{u}_i\,, \tag{2}$$

as illustrated in Fig. 2c of the main text. The non-trivial phase difference $\phi_j - \phi_i$ then leads to a complex nearest-neighbor hopping. With hopping elements defined in anticlockwise direction around the elementary triangular plaquettes of the Kagome lattice (see Figs. 1 and 2 of the main text), we obtain two decoupled Haldane-like Kagome lattice models — one for each component $u$ and $v$ — with hopping terms

$$t_u = t\left(1 + \left(\frac{g}{2\Omega}\right)^2 \mathrm{e}^{i2\pi/3}\right), \quad t_v = -t\left(1 + \left(\frac{g}{2\Omega}\right)^2 \mathrm{e}^{-i2\pi/3}\right). \tag{3}$$

The total effective flux per triangular plaquette is then given by

$$\Phi_u = 3\arg\left[\left(1 + \left(\frac{g}{2\Omega}\right)^2 \mathrm{e}^{i2\pi/3}\right)\right] = 3\arctan\left[\frac{\sqrt{3}g^2}{8\Omega^2 - g^2}\right] \approx \frac{3\sqrt{3}}{2}\left(\frac{g}{2\Omega}\right)^2, \tag{4}$$

with a corresponding opposite flux for hole-like Bogoliubons, i.e., $\Phi_v = -\Phi_u$. For fluxes $\Phi_u$ that are not multiples of $\pi$, the time-reversal symmetry of the effective Haldane model is broken and topological gaps are expected to open at the band touchings occurring at the high-symmetry points $\Gamma$ and $K, K'$ (see Fig. 1 and Ref. [1]). This is indeed confirmed by direct numerical implementation of the tight-binding model (1), as detailed below.

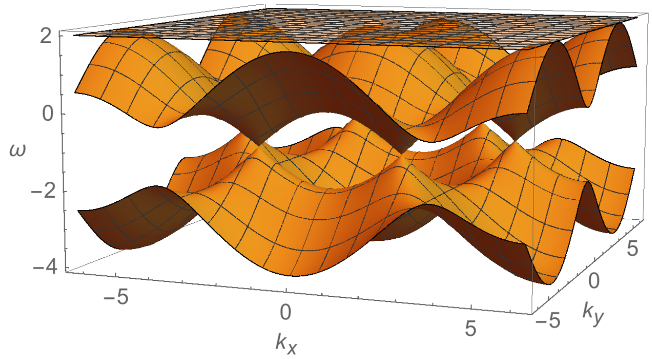


FIG. 1. Kagome tight-binding spectrum of particle-like Bogoliubons (component $u$) for $\Omega = 0$ and $t = 1$, in the absence of any coupling $g$ with hole-like Bogoliubons (component $v$).

**Size of the topological gaps**

To determine the size of the expected topological gaps, we consider a system with periodic boundary conditions and diagonalize the tight-binding Hamiltonian (1). This can be done by choosing a triangular unit cell $\hat{\mathbf{u}}_i = (\hat{u}_A, \hat{u}_B, \hat{u}_C)_i$ (as defined in Fig. 2b of the main text) and moving to momentum space by a Fourier transformation $\hat{\mathbf{u}}_i = \sum_{\mathbf{k}} \hat{\mathbf{u}}_{\mathbf{k}} \mathrm{e}^{i\mathbf{k}\mathbf{r}_i}$. The Hamiltonian in the sector corresponding to $u$ then takes the form

$$H_{uu} = \begin{pmatrix} \Omega & -t\left(1+\mathrm{e}^{-i\left(k_x-\sqrt{3}k_y\right)/2}\right) & -t\left(1+\mathrm{e}^{-ik_x}\right) \\ -t\left(1+\mathrm{e}^{i\left(k_x-\sqrt{3}k_y\right)/2}\right) & \Omega & -t\left(1+\mathrm{e}^{-i\left(k_x+\sqrt{3}k_y\right)/2}\right) \\ -t\left(1+\mathrm{e}^{ik_x}\right) & -t\left(1+\mathrm{e}^{i\left(k_x+\sqrt{3}k_y\right)/2}\right) & \Omega \end{pmatrix}, \tag{5}$$

with a similar block $H_{vv}$ obtained by taking $\Omega \to -\Omega$ and $t \to -t$. Momentum is measured in units of $1/a$, where $a$ is the lattice constant which corresponds to the distance between triangular unit cells (or twice the distance between nearest-neighboring sites; see Fig. 2b of the main text). In the decoupled system (i.e., with $g = 0$), $H_{uu}$ describes a well-known Kagome tight-binding lattice model. Eigenvalues are given by $\omega_1(\mathbf{q}) = \omega - 2t$ and $\omega_{2/3}(\mathbf{q}) = \omega + t\,(1 \pm \xi)$, where $\xi = \left(3 + 2\cos(k_x) + 4\cos(k_x/2)\cos\left(\sqrt{3}k_y/2\right)\right)^{1/2}$; the corresponding spectrum is shown in Fig. 1. Most importantly, the model exhibits degeneracies at high symmetry points of the Brillouin zone, with Dirac cones at $K = (4\pi/3, 0)$ and $K' = (2\pi/3, 2\pi/\sqrt{3})$, and a quadratic band touching at $\Gamma = (0, 0)$.

The topological gaps appear exactly at these degeneracies. We can therefore focus on the high symmetry points. In this regime, the eigenvectors are best expressed in terms of the basis $|s\rangle = (1,1,1)/\sqrt{3}$, $|\circlearrowleft\rangle = (1, \mathrm{e}^{i2\pi/3}, \mathrm{e}^{-i2\pi/3})$, $|\circlearrowright\rangle = (1, -\mathrm{e}^{i2\pi/3}, \mathrm{e}^{i2\pi/3})$. Applying the corresponding basis transformation

$$U = \frac{1}{\sqrt{3}} \begin{pmatrix} 1 & 1 & 1 \\ 1 & \mathrm{e}^{i\frac{2\pi}{3}} & \mathrm{e}^{-i\frac{2\pi}{3}} \\ 1 & \mathrm{e}^{-i\frac{2\pi}{3}} & \mathrm{e}^{i\frac{2\pi}{3}} \end{pmatrix}$$

to the sector $u$ of the Hamiltonian gives

$$U^\dagger H_{uu}(\mathbf{k}=K)U = \begin{pmatrix} \Omega - t & 0 & 0 \\ 0 & \Omega - t & 0 \\ 0 & 0 & \Omega + 2t \end{pmatrix}, \quad U^\dagger H_{uu}(\mathbf{k}=\Gamma)U = \begin{pmatrix} \Omega - 4t & 0 & 0 \\ 0 & \Omega + 2t & 0 \\ 0 & 0 & \Omega + 2t \end{pmatrix},$$

with similar results for the sector $v$. Applying the transformation $U$ to the off-diagonal blocks coupling $u$ and $v$ yields

$$U^\dagger H_{uv} U = g \begin{pmatrix} 0 & 0 & 1 \\ 1 & 0 & 0 \\ 0 & 1 & 0 \end{pmatrix}, \quad U^\dagger H_{vu} U = -g \begin{pmatrix} 0 & 1 & 0 \\ 0 & 0 & 1 \\ 1 & 0 & 0 \end{pmatrix}.$$

The corresponding full Hamiltonian can then be exactly diagonalized. For small coupling $g$, the associated spectrum is real and eigenvalues come in pairs with opposite signs (see, e.g., Fig. 2a of the main text). The positive part of

the spectrum is given by the eigenvalues $\omega_1(K) = \sqrt{(\Omega - t)^2 - g^2}$ and $\omega_{2/3}(K) = \sqrt{(\Omega + t/2)^2 - g^2} \pm 3/2t$, as well as $\omega_1(\Gamma) = \sqrt{(\Omega + 2t)^2 - g^2}$ and $\omega_{2/3}(\Gamma) = \sqrt{(\Omega - t)^2 - g^2} \pm 3t$. The corresponding topological gaps are given by

$$\Delta_K = \omega_3(K) - \omega_1(K) \approx \frac{3g^2 t}{4(\Omega - t)(\Omega + t/2)}, \tag{6}$$

$$\Delta_\Gamma = \omega_1(\Gamma) - \omega_2(\Gamma) \approx \frac{3g^2 t}{2(\Omega - t)(\Omega + 2t)}, \tag{7}$$

where we have assumed $g \ll \Omega - t$ ($g \ll \Omega + 2t$) in the second step of each line.

### Numerics

To compute the spectrum presented in Fig. 2a of the main text, we considered periodic boundary conditions in $x$-direction and vanishing boundary conditions in $y$-direction. The resulting effective one-dimensional tight-binding model then consists of on-site terms $A$ and hopping terms in the $y$-direction $B$ with

$$A = \begin{pmatrix} A_{uu} & A_{uv} \\ A_{vu} & A_{vv} \end{pmatrix}, \quad B = \begin{pmatrix} B_{uu} & 0 \\ 0 & B_{vv} \end{pmatrix}, \text{ where} \tag{8}$$

$$A_{uu} = \begin{pmatrix} \Omega & -t & -t(1 + \mathrm{e}^{-ik_x}) \\ -t & \Omega & -t \\ -t(1 + \mathrm{e}^{ik_x}) & -t & \Omega \end{pmatrix}, \; A_{uv} = g \begin{pmatrix} 1 & 0 & 0 \\ 0 & \mathrm{e}^{i2\pi/3} & 0 \\ 0 & 0 & \mathrm{e}^{-i2\pi/3} \end{pmatrix}, \; A_{vv} = -A_{uu}, \;\; A_{vu} = -A_{uv}^\dagger \tag{9}$$

$$B_{uu} = -t \begin{pmatrix} 0 & \mathrm{e}^{-ik_x/2} & 0 \\ 0 & 0 & 0 \\ 0 & \mathrm{e}^{ik_x/2} & 0 \end{pmatrix}, \; B_{vv} = -B_{uu}. \tag{10}$$

As expected, the spectrum exhibits topological gaps at the high symmetry points (see Fig. 2a of the main text).

## TOPOLOGICAL BOGOLIUBONS IN EXCITON-POLARITON SYSTEMS

In this section, we present in more details the practical realization of our scheme using exciton-polaritons in planar semiconductor microcavities. We first derive the relevant spin-dependent Bogoliubov equation and outline a suitable pumping scheme to create a condensate with the Kagome intensity pattern and vortex structure used in our scheme, as discussed in the main text. We then detail the method and parameters used to derive the spectrum presented in Fig. 3a of the main text.

### Spin-dependent Bogoliubov equation

We start from the standard spin-dependent Gross-Pitaevskii equation (or nonlinear Schrödinger equation) describing the dynamics of exciton-polaritons in planar semiconductor microcavities [2]. Polaritons can have a spin projection (or circular polarization) $\sigma = \pm 1$ along the $z$-direction perpendicular to the plane. Under coherent pumping, the corresponding mean-field wavefunction $\psi_\sigma(\mathbf{x}, t)$ evolves according to

$$i\partial_t \psi_\sigma = \left(\omega_d(-i\boldsymbol{\nabla}) + \alpha_1 |\psi_\sigma|^2 + \alpha_2 |\psi_{-\sigma}|^2 + V(\mathbf{x}) - i\gamma\right) \psi_\sigma + p_\sigma f(\mathbf{x}) e^{-i\omega_0 t}, \tag{11}$$

where $\omega_d(-i\boldsymbol{\nabla})$ describes the polariton dispersion, $\alpha_1$ and $\alpha_2$ denote the strength of interactions between polaritons of parallel and opposite spins, respectively, and $\gamma$ is the polariton decay rate. Polaritons of parallel spin typically repel each other (i.e., $\alpha_1 > 0$), while the interaction between polaritons of opposite spins is usually weaker and attractive (i.e., $\alpha_2 < 0$ with $|\alpha_2| < \alpha_1$) [2]. We assume that polaritons of both spins are injected simultaneously using an elliptically polarized incident field (or "pump") with frequency $\omega_0$ and spatial profile $f(\mathbf{x})$. The ellipticity is determined by the positive parameters $p_{\pm\sigma}$ which control the relative intensity between spin components.

To simplify our analysis, we focus on the slowly-varying field $\phi_\sigma(\mathbf{x}, t) \equiv \psi_\sigma(\mathbf{x}, t) e^{i\omega_0 t}$. The relevant Gross-Pitaevskii equation then becomes

$$i\partial_t \phi_\sigma = \left(\omega_d(-i\boldsymbol{\nabla}) - \omega_0 + \alpha_1 |\phi_\sigma|^2 + \alpha_2 |\phi_{-\sigma}|^2 + V(\mathbf{x}) - i\gamma\right) \phi_\sigma + p_\sigma f(\mathbf{x}), \tag{12}$$

where the explicit time dependence $e^{i\omega_0 t}$ has been replaced by the detuning $\omega_d(-i\boldsymbol{\nabla}) - \omega_0$. Next we consider fluctuations of the form

$$\phi_\sigma(\mathbf{x}, t) = \phi_{0,\sigma}(\mathbf{x}, t) + u_\sigma(\mathbf{x})e^{-i\omega t} + v_\sigma^*(\mathbf{x})e^{i\omega^* t}, \tag{13}$$

where $\phi_{0,\sigma}(\mathbf{x})$ is the stationary solution of Eq. (12), $u_\sigma(\mathbf{x})$ and $v_\sigma(\mathbf{x})$ are (in general complex) functions determining the spatial profile of the fluctuations, and $\omega$ is the frequency of the perturbations, which is kept complex in order to capture potential instabilities [3]. Plugging the above expression into Eq. (12) and neglecting second-order terms in $u_\sigma$ and $v_\sigma$ then yields

$$\begin{aligned} \omega u_\sigma(\mathbf{x})e^{-i\omega t} - \omega^* v_\sigma^*(\mathbf{x})e^{i\omega^* t} = &\left(\omega_d(-i\boldsymbol{\nabla}) - \omega_0 + 2\alpha_1|\phi_{0,\sigma}|^2 + \alpha_2|\phi_{0,-\sigma}|^2 + V(\mathbf{x}) - i\gamma\right)\left(u_\sigma(\mathbf{x})e^{-i\omega t} + v_\sigma^*(\mathbf{x})e^{i\omega^* t}\right) \\ &+ \alpha_1\phi_{0,\sigma}^2\left(u_\sigma^*(\mathbf{x})e^{i\omega^* t} + v_\sigma(\mathbf{x})e^{-i\omega t}\right) \\ &+ \alpha_2\phi_{0,-\sigma}^*\phi_{0,\sigma}\left(u_{-\sigma}(\mathbf{x})e^{-i\omega t} + v_{-\sigma}^*(\mathbf{x})e^{i\omega^* t}\right) \\ &+ \alpha_2\phi_{0,-\sigma}\phi_{0,\sigma}\left(u_{-\sigma}^*(\mathbf{x})e^{i\omega^* t} + v_{-\sigma}(\mathbf{x})e^{-i\omega t}\right). \end{aligned} \tag{14}$$

We consider fluctuations with fixed $\sigma$, for simplicity, such that $u_{-\sigma}(\mathbf{x}) = v_{-\sigma}(\mathbf{x}) = 0$. Collecting terms oscillating at the same frequency then yields the desired spin-dependent Bogoliubov equation

$$\begin{pmatrix} \omega'(\mathbf{x}) - i\gamma & \alpha_1\phi_{0,\sigma}(\mathbf{x})^2 \\ -\alpha_1\phi_{0,\sigma}(\mathbf{x})^{*2} & -\omega'(\mathbf{x}) - i\gamma \end{pmatrix}\begin{pmatrix} u_\sigma(\mathbf{x}) \\ v_\sigma(\mathbf{x}) \end{pmatrix} = \omega\begin{pmatrix} u_\sigma(\mathbf{x}) \\ v_\sigma(\mathbf{x}) \end{pmatrix}, \tag{15}$$

where we have defined $\omega'(\mathbf{x}) \equiv \omega_d(-i\boldsymbol{\nabla}) - \omega_0 + 2\alpha_1|\phi_{0,\sigma}|^2 + \alpha_2|\phi_{0,-\sigma}|^2 + V(\mathbf{x})$ using similar notations as in the main text.

### Scheme for topological Bogoliubons

The diagonal part of equation (15) describes "particle and hole-like" Bogoliubov excitations with opposite dispersions $\pm\omega'(\mathbf{x})$ (and the same decay rate $\gamma$). Up to an energy shift $-\omega_0$, the dispersion $\omega'(\mathbf{x})$ corresponds to that of particles with dispersion $\omega_d(-i\boldsymbol{\nabla})$ in an effective potential of the form $2\alpha_1|\phi_{0,\sigma}|^2 + \alpha_2|\phi_{0,-\sigma}|^2 + V(\mathbf{x})$, which depends on the interaction strengths $\alpha_1$ and $\alpha_2$ as well as the intensity of the spin components $\phi_{0,\sigma}$ and $\phi_{0,-\sigma}$ of the underlying condensate.

To create topological Bogoliubov excitations, we start from these uncoupled particle- and hole-like Bogoliubov excitations, in a regime where they are mostly off-resonant [4], and introduce the off-diagonal coupling terms $\pm\alpha_1\phi_{0,\sigma}(\mathbf{x})^{(*)2}$ appearing in Eq. (15). As discussed in the main text, this off-diagonal coupling, which depends on the phase of the underlying condensate, is crucial to generate topological states: its phase allows for time-reversal symmetry breaking and its amplitude ultimately limits the size of the topological gaps that can be obtained. To "feel" this coupling in an optimal way, particle- and hole-like excitations must "live" in regions of space where the intensity of the underlying condensate is maximal, such that the amplitude $\alpha_1|\phi_{0,\sigma}(\mathbf{x})|^2$ of the coupling is large. This can be achieved in two (possibly complementary) ways: (i) by introducing an external potential $V(\mathbf{x})$ that localizes excitations at the intensity maxima of the condensate, or/and (ii) by focusing on a particular spin-component and using the other one to induce the required potential optically. Here we set $V(\mathbf{x}) = 0$ and focus on this second option, which does not allow to create topological Bogoliubons simultaneously in both spin components, but has the practical advantage of not requiring any external potential. In that case the effective potential seen by Bogoliubov excitations with spin $\sigma$ reduces to $2\alpha_1|\phi_{0,\sigma}|^2 + \alpha_2|\phi_{0,-\sigma}|^2$.

Let us now describe our pumping scheme. To generate the "Kagome vortex lattice" considered in the main text (see Fig. 1 thereof), we consider, e.g., a pumping field that can be described as a superposition of six plane-wave components of frequency $\omega_0$, with in-plane wave vectors and phases defined as

$$\begin{aligned} k_1 &= k_0(\sqrt{3}/2, 1/2), & \phi_1 &= 0; \\ k_2 &= k_0(0, 1), & \phi_2 &= 0; \\ k_3 &= k_0(-\sqrt{3}/2, 1/2), & \phi_3 &= 0; \\ k_4 &= k_0(-\sqrt{3}/2, -1/2), & \phi_4 &= 2\pi/3; \\ k_5 &= k_0(0, -1), & \phi_5 &= 0; \\ k_6 &= k_0(\sqrt{3}/2, -1/2), & \phi_6 &= -2\pi/3, \end{aligned} \tag{16}$$

such that $p_\sigma f(\mathbf{x})e^{-i\omega_0 t} = p_\sigma \sum_{n=1}^{6} \exp[i(\mathbf{k}_n \cdot \mathbf{x} - \omega_0 t + \varphi_n)]$, i.e., $f(\mathbf{x}) \equiv \sum_{n=1}^{6} \exp[i(\mathbf{k}_n \cdot \mathbf{x} + \varphi_n)]$. The pump spatial profile $f(\mathbf{x})$ exhibits the desired vortex lattice structure, with vortex-antivortex pairs and intensity maxima forming a Kagome lattice structure (as shown in Fig. 1 of the main text). The corresponding lattice constant is determined by the norm $k_0$, i.e., $a = 2\pi/(\sqrt{3}/2\, k_0)$, and the direction of rotation of vortices can be reversed by taking $\phi_n \to -\phi_n$, thereby changing the chirality of the system.

In the absence of interactions ($\alpha_1, \alpha_2 = 0$), the Gross-Pitaevskii equation (12) gives rise to stationary polariton wavefunctions $\phi_{0,\sigma}(\mathbf{x})$ and $\phi_{0,-\sigma}(\mathbf{x})$ with the same spatial profile as the pumping field (and intensity controlled by $p_\sigma$ and $p_{-\sigma}$). Here we assume that the pump intensity (polariton density) is low enough to remain in the linear regime where polariton interactions do not drastically modify the phase and intensity pattern imprinted by the pump field (so as to avoid, in particular, typical multistability effects [3]). In that case the stationary fields $\phi_{0,\pm\sigma}(\mathbf{x})$ exhibit a similar Kagome vortex lattice as the pump profile $f(\mathbf{x})$, as we have verified in the numerical analysis detailed below.

## Numerics

We now detail the method and parameters used to obtain the spectrum presented in Fig. 3a of the main text. To provide the most accurate estimate for the size of the topological gap achievable in practice, we computed the Bogoliubov excitations spectrum using parameters from existing experiments [5] without relying on any tight-binding approximation. Specifically, we considered a strip geometry defined by periodic boundary conditions in the $x$-direction and open (Dirichlet) boundary conditions in the $y$-direction. We derived the Bogoliubov spectrum by expressing the solutions of Eq. (15) in Bloch form, i.e., $u_\sigma(x,y) = \exp(ik_x x)\tilde{u}_\sigma(x,y)$, with $\tilde{u}_\sigma(x,y)$ periodic in $x$ (and similarly for $v_\sigma(x,y)$). The periodicity of $\tilde{u}_\sigma(x,y)$, $\tilde{v}_\sigma(x,y)$ and $\phi_{0,\pm\sigma}(x,y)$ then allowed us to expand all terms appearing in Eq. (15) as Fourier sums, leading to an eigenvalue problem that can be solved straightforwardly to find the spectrum $\omega(k_x)$. We followed a similar wave-expansion method to first compute the stationary fields $\phi_{0,\pm\sigma}(x,y)$ resulting from Eq. (12).

To produce the results presented in Fig. 3a of the main text, we focused on the lower polariton branch (assuming that the energy separation between lower and upper polariton branches is larger than all relevant energy scales for Bogoliubov excitations), and approximated the corresponding dispersion as $\omega_d(-i\boldsymbol{\nabla}) \approx -\hbar\nabla^2/(2m_{\text{eff}})$. Parameters were chosen as (see Ref. [5]):

- Lattice constant $a = 3\mu$m;
- Polariton effective mass $m_{\text{eff}} = 10^{-4} m_0$, where $m_0$ is the free electron mass;
- Interaction strength $\alpha_1 = 2.4 \cdot 10^{-3}\text{meV}\mu\text{m}^2/\hbar$; $\alpha_2 = -0.2\alpha_1$;
- Polariton decay rate $\gamma = 0.2\text{ps}^{-1}$ (not visible in Fig. 3a of the main text showing the real part of the Bogoliubov spectrum, but taken into account in the discussion thereof);
- Pump frequency $\omega_0 = -2.2\text{meV}/\hbar$ (relative to the bottom of the lower polariton dispersion $\omega_d(-i\boldsymbol{\nabla})$);
- $p_\sigma^2 = 1\text{Wcm}^{-2}/\hbar$; $p_{-\sigma} = 100 p_\sigma$.

[1] K. Ohgushi, S. Murakami, and N. Nagaosa, Phys. Rev. B **62**, R6065 (2000).
[2] I. Carusotto and C. Ciuti, Rev. Mod. Phys. **85**, 299 (2013).
[3] I. Carusotto and C. Ciuti, Phys. Rev. Lett. **93**, 166401 (2004).
[4] The off-resonant regime is crucial to obtain Bogoliubov excitations that are stable, with no positive imaginary part in the corresponding spectrum. Such a regime can easily be reached, e.g., by tuning the pump frequency $\omega_0$.
[5] F. Manni, K. G. Lagoudakis, T. C. H. Liew, R. André, V. Savona, and B. Deveaud, Nat. Comm. **3**, 1309 (2012).
